# Supplementary material for: UniClawBench: A Universal Benchmark for Proactive Agents on Real-World Tasks
Source: arXiv:2607.08768 source file (2026-07-09)
Supplement: Supplementary file 1 [file A_task_format.tex]

A UniClawBench task is generally defined by two files: a single task
declaration written in YAML that fixes the public contract, and a
hidden \texttt{eval\_rule.md} that specifies the rubric. The executor
sees only the \texttt{task} field rendered into a runtime prompt; the
supervisor sees both files and treats the eval rule as the canonical
scoring contract. Appendix~\ref{app:format:yaml} gives the YAML template that fixes
the public contract; Appendix~\ref{app:format:fields} walks through the
semantics of each field; and Appendix~\ref{app:format:eval} specifies the
nine-section schema of the hidden eval rule.

\subsection{Task YAML Template}\label{app:format:yaml}

\begin{clawcode}[title={Task YAML Template},label={lst:format:yaml}]
task_id: task_NNN_short_slug
category: <suite_name>
agent_sys: openclaw
agent_id: main
model: claude-opus-4.6

timeout_seconds: 1200
max_total_seconds: 1800
success_threshold: 0.90

task: |
  <natural-language request shown to the executor>

task_snapshot: |
  <parallel-safe variant>

references:
  - references/eval_rule.md
  - references/ground_truth.json
  - ...

sources:
  - <relative_path>

skills:
  - <skill_id>

services:
  - name: <service>
    path: <subdir>
    start: bash install.sh
    oneshot: true

pre_exec:
  - ops/populate.py
pre_exec_parallel_safe: true

codex:
  max_user_followups: 2
  user_simulator:
    policy: |
      <override of the default user-simulator policy>
  supervisor:
    instructions: |
      <task-specific addendum to the default supervisor instructions>
\end{clawcode}

\subsection{Field Semantics}\label{app:format:fields}

\paragraph{Basic definition.}
\texttt{task\_id} is unique within the suite and is also the file
stem. \texttt{category} is one of the five task dimensions from the main
paper. \texttt{agent\_sys}, \texttt{agent\_id}, and \texttt{model}
record the \emph{default} executor binding when the task is
dispatched without an override; cross-architecture and cross-model
sweeps override these at runtime.

\paragraph{Lifecycle.}
\texttt{timeout\_seconds} bounds a single executor cycle.
\texttt{max\_total\_seconds} bounds the whole-attempt wall clock
across all cycles, excluding supervisor and user-simulator turns.
\texttt{success\_threshold} is the minimum supervisor score that
records the attempt as \texttt{Pass}. The cycle count is bounded separately by
\texttt{codex.max\_user\_followups}.

\paragraph{Task prompt.}
\texttt{task} is the literal natural-language request the executor
receives, wrapped in a small runtime preamble that surfaces workspace
paths and installed skills. \texttt{task\_snapshot} is an optional
snapshot version that consumes snapshot data
instead of a live API.

\paragraph{Injections.}
\texttt{sources} lists files placed under the executor's workspace mount.
\texttt{skills} lists declared skills; the eval rule for a
skill-usage task typically requires transcript evidence that the
declared skill was actually consulted. \texttt{services} entries are
docker-compose-style bootstrap services started before the executor's
first turn (databases, mock APIs, GUI app installers).
\texttt{pre\_exec} scripts run once after services are healthy and
typically populate session-specific fixture state into live API.
\texttt{references} are hidden judging assets placed under the
supervisor's workspace and never copied into the executor container.

\paragraph{Supervisor and user simulator.}
The \texttt{codex} block configures the closed-loop interaction.
\texttt{max\_user\_followups} bounds the number of follow-up cycles
allowed before the runner forcibly closes the attempt.
\texttt{codex.user\_simulator.policy} overrides the default
user-simulator behavior policy when a task needs a non-standard
interaction style (e.g.\ a deliberately terse user, a user with a
specific persona constraint).
\texttt{codex.supervisor.instructions} appends a task-specific
addendum to the default supervisor template, used to highlight
checkpoints that are easy to miss without explicit attention or to
narrow down what counts as evidence for an unusual artifact.
Both blocks are optional; when absent, the defaults from
Appendix~\ref{app:prompts} apply.

\subsection{Eval Rule (\texttt{eval\_rule.md}) Format}\label{app:format:eval}

Every task ships a hidden Markdown rubric at
\texttt{references/eval\_rule.md}. The rubric follows a fixed
nine-section schema: \S1--\S4 establish the contract, \S5--\S6
define scoring, and \S7--\S9 cover lifecycle policy and asset
bookkeeping. The supervisor prompt instructs the supervisor to score
using the lines that appear in \S5 and \S6, and other parts guide the
understanding and flexible judgment.

\begin{clawschema}[title={Eval rule schema},label={lst:format:eval}]
\schemaitem{1. Grading Philosophy}{States what the task tests, what
  is rewarded, and what should not be penalized. Notes the role of
  declared skills.}

\schemaitem{2. Task Contract}{Restates the public prompt with
  deliverable paths pinned, and separates hard requirements (must
  produce) from soft requirements (must follow these formats).}

\schemaitem{3. Source-Selection and Target-Resolution Rules}{How the
  supervisor maps executor artifacts to ground-truth entities --
  alias rules, filename-stem variants, numeric tolerance bands.}

\schemaitem{4. Ground-Truth Snapshot}{Pointer to ground-truth files
  with canonical entity counts and any must-not-appear entities for
  negative checkpoints.}

\schemaitem{5. Checkpoint Rubric}{Numbered scoring lines whose
  weights sum to 1.00. Each is boolean, graded, or count-based. The
  supervisor scores using only these lines.}

\schemaitem{6. Scoring Policy \& Score Caps}{Hard ceilings applied
  after the \S5 sum. A cap is a maximum and cannot raise a \S5 sum
  that is already lower.}

\schemaitem{7. Continue vs Fail Guidance}{Score banding for the
  \texttt{pass} / \texttt{continue} / \texttt{fail} verdicts. The
  mid-band lets the supervisor request one focused follow-up.}

\schemaitem{8. Hidden Reference Assets}{Inventory of
  supervisor-only files; reaffirms that none are surfaced to the
  executor or user simulator.}

\schemaitem{9. Dynamic Content Note}{Whether the task is offline
  (static fixture) or live (consumes an external page that may
  shift between captures), with reconciliation rules for live
  tasks.}
\end{clawschema}
