# Supplementary material for: UniClawBench: A Universal Benchmark for Proactive Agents on Real-World Tasks
Source: arXiv:2607.08768 source file (2026-07-09)
Supplement: Supplementary file 2 [file B_suite_examples.tex]

This section lists representative task examples from each suite. For
every task dimension we show two prompts. Each prompt is the literal
natural-language \texttt{task} field that the executor sees at
runtime; the surrounding YAML schema follows
Appendix~\ref{app:format}.

\subsection{Skill Usage}\label{app:examples:skill}

Tasks here ship several declared skills and require the executor to actually
consult it. The agent's job is to discover the skill, follow its
\texttt{SKILL.md} entry-point, and apply the right tool to the
provided data.

\begin{clawcode}[title={\texttt{task\_05\_org\_chart\_mermaid}}]
Our CEO asked for a governance visualization she can drop into her
board deck, and I need to pull it from the proxy statement. The
excerpt lives at
/tmp_workspace/clawbench/sources/alphabet_def14a_excerpt.md -- use the
Mermaid diagramming skill to turn it into a clean org chart. She wants
to see the actual reporting hierarchy -- the solid lines from each
current director to the board and from each non-CEO executive officer
to the executive roster -- who sits on which committee across the
audit, compensation, governance, and executive committees, and the
dotted advisory or observer relationships that aren't formal seats.
We also need who chairs what, and any seats that are vacant, interim,
advisor-only, or recently filled.

Please render it as Mermaid using graph TD or flowchart TD in
/tmp_workspace/results/org.mmd, and produce an SVG rendering at
/tmp_workspace/results/org.svg. Use solid arrows for board and
executive roster relationships that are explicitly supported by the
excerpt, dotted arrows for committee memberships and any non-voting
advisor or observer relationships, and group each committee as a
subgraph. Distinguish committee chairs visually from regular members
-- shape or styling is fine. Treat each person as a single node; if
someone holds multiple roles, draw their relationships from that one
node rather than duplicating them. Anyone listed as recently-departed
should not appear as a current node.

Also save /tmp_workspace/results/governance_matrix.csv so my chief of
staff can review the extraction without reading Mermaid. Use columns:
person, source_role, governance_group_or_board, committee,
committee_role, edge_type, source_quote.
\end{clawcode}

\begin{clawcode}[title={\texttt{task\_19\_github\_activity\_digest}}]
I missed the last two weeks of activity on clawbench-activity-fixture
and need to catch up before the maintainer sync. Build me a 16-day
activity digest covering 2026-04-10 through 2026-04-25 inclusive --
use the GitHub skill in our workspace for the API calls. Authenticate
with the \$GITHUB_TOKEN environment variable and hit the live GitHub
REST API directly via the gh CLI or curl against api.github.com. Do
not rely on any local cache or pre-exported snapshot file under
/tmp_workspace/clawbench for this run; everything must come from a
fresh API pull covering merged PRs, closed-unmerged PRs, closed
issues, and commits in that window.

A few entries in this fixture repo may have been imported by an
automation account. When a PR or issue body, or a commit message,
includes an explicit pseudo-user or planned-date note, use that note
as the contributor and date for the digest instead of the automation
account's login or the rebuild timestamp.

Save /tmp_workspace/results/digest.md grouped by contributor. For
each contributor show: PRs merged, PRs closed without merge, issues
closed, and commit count. Add a Follow-up Flags section for activity
that looks risky or needs a maintainer follow-up, including every
closed-unmerged PR and any revert PR or revert commit. End with a
Highlights section listing the 5 most recent merged PRs or closed
issues in the window, newest first. When two highlight events share
the same date, list the higher-numbered activity first so number 27
comes before number 13; if the numbers also tie, list the issue
before the pull request.

Also save /tmp_workspace/results/activity_index.csv with columns
activity_type,number_or_sha,title_or_message,contributor,activity_date,status
covering every merged PR, closed-unmerged PR, closed issue, and
commit in the 16-day window so I can sort and filter it later. Cover
the full set of contributors and activity, not a partial sample.
\end{clawcode}

\subsection{Exploration}\label{app:examples:exploration}

Tasks here are open-ended audits or refactors over noisy and
potentially misleading inputs. The agent must investigate multiple
choices, reject incorrect alternatives, and document negative
evidence to distinguish real exploration from a guessed conclusion.

\begin{clawcode}[title={\texttt{task\_01\_zshrc\_prompt\_refactor}}]
Your goal is to refactor the injected legacy `.zshrc` into a
maintainable, low-noise, verifiable zsh configuration. The input file
is at `/tmp_workspace/sources/existing_zshrc`. This is not about
writing a new prompt snippet from scratch; you must preserve the real
behaviors from the original config and eliminate the conflicts it
already contains.

Start by auditing the legacy config: identify duplicate PATH entries,
duplicate PROMPT/RPROMPT definitions, `precmd` overrides, Oh My
Zsh/plugin load order issues, conda/nvm initialization placement, and
any fragments that may produce side effects in interactive vs.
non-interactive shells. Then produce the final `.zshrc`: preserve
aliases, plugins, PATH prepends, the conda hook, and nvm sourcing;
the prompt should be concise, showing the current path and git
status, but must not display username, hostname, time,
Python/Node/Ruby runtime, full deep paths, or Nerd Font-only glyphs
by default.

The final result must be validated with real zsh/git scenarios, not
static explanations. Cover all eight scenarios: plain shell, git
clean, git dirty, detached HEAD, rebase/merge state, deep path,
Python venv active, and non-interactive `zsh -fc true`. Document
that startup time has not degraded noticeably.

Save:
- `/tmp_workspace/results/zshrc_final`
- `/tmp_workspace/results/zsh_prompt_audit.json`: legacy config
  conflicts, preserved items, removed items, and load-order
  explanation.
- `/tmp_workspace/results/zsh_prompt_patch_notes.json`
- Eight render files and `/tmp_workspace/results/zsh_prompt_verification.log`.
\end{clawcode}

\begin{clawcode}[title={\texttt{task\_18\_license\_provenance\_audit}}]
Perform an offline open-source license provenance audit. Do not go
online; the inputs are at:

    /tmp_workspace/sources/license_audit/

Each package has a package.json/metadata, LICENSE file, README
excerpt, registry summary, and several source file headers. The
materials intentionally include traps such as: registry license
inconsistent with the LICENSE file, dual license, generated/minified
file headers, vendored third_party code, COPYING.LESSER vs. GPL
confusion, and misleading README badges. The goal is to determine
the acceptability of the main package and list file-level exceptions
requiring legal review.

Company policy: MIT/Apache-2.0/BSD-2-Clause/BSD-3-Clause/ISC are
allowed; MPL-2.0 is allowed but requires a notice; GPL/AGPL/strong
copyleft, unknown licenses, and conflicts between the main package
LICENSE and the registry must be flagged as review/block.

Save the following:
- `/tmp_workspace/results/license_audit_summary.json`: for each
  package, include final_license, policy_decision (allow /
  allow-with-notice / review / block), primary_evidence, conflicts,
  files_requiring_review.
- `/tmp_workspace/results/license_file_matrix.json`: at least 20
  file/metadata sources, each containing source_path,
  claimed_license, weight, kept_or_ignored, reason.
- `/tmp_workspace/results/license_rejection_traps.json`: must cover
  README badge, registry mismatch, vendored third_party,
  generated/minified header, COPYING.LESSER/GPL confusion, and
  dual license.
- `/tmp_workspace/results/license_method.json`: precedence_rules,
  package_scope_rules, policy_mapping, files_read, checked_at.
- `/tmp_workspace/results/audit_package_licenses.py` and run log.
\end{clawcode}

\subsection{Long-Context Reasoning}\label{app:examples:long-context}

Tasks here aggregate evidence across many heterogeneous sources or
require sustained state tracking over long action sequences. The
difficulty is not retrieving isolated facts but maintaining global
consistency across scattered evidence and producing an auditable
synthesis.

\begin{clawcode}[title={\texttt{task\_03\_slack\_openclaw\_assistant\_setup}}]
I currently use Slack on my phone, and OpenClaw is already installed
locally, but this OpenClaw assistant has not yet been connected inside
Slack.

I watched this video and it seems that Slack integration should be
possible: https://www.youtube.com/watch?v=9QpSkGnfKMk . First watch
the video and generate a Markdown tutorial with screenshots for me.
Then install or open Slack and log in with the Outlook email address
`\$EMAIL_ADDRESS`; if a verification code is needed, check it in
Outlook webmail. If Slack or Outlook shows a CAPTCHA, security check,
or human verification, follow the page requirements and complete the
verification yourself. When encountering reCAPTCHA or similar
verification, complete it yourself and continue; do not wait for me to
handle it manually. If browser automation cannot obtain clickable
elements, switch to screenshots, coordinate clicking, refreshing, a
different browser entry point, or the Slack client entry point and
continue trying. Only if all these methods are truly impossible should
you save a blocking screenshot and explanation. After logging in,
configure or reset an OpenClaw bot/assistant entry and connect local
OpenClaw to Slack.

Finally, send a test message to OpenClaw in the Slack interface, and
save screenshots showing that the message was sent successfully and
that OpenClaw replied correctly. Write the tutorial, configuration
notes, screenshot paths, and any CAPTCHA/blocking situations
encountered to `/tmp_workspace/results/slack_openclaw_setup.md`. Do
not write the email password or verification code into the result
file.
\end{clawcode}

\begin{clawcode}[title={\texttt{task\_07\_santa\_monica\_trip\_budget}}]
I want to go to Santa Monica in Los Angeles with a friend for a long
weekend in July 2026. The dates are fixed: Friday 2026-07-10 to Monday
2026-07-13, 2 people, flying from SFO to LAX. Please actually research
and create a complete budget and itinerary plan, but do not pay, book
tickets, book hotels, rent a car, reserve restaurants, or submit any
irreversible order. Save all screenshots and documents to
`/tmp_workspace/results/`.

For flights, only consider United nonstop. The outbound flight must
depart SFO for LAX on 2026-07-10 between 09:00 and 11:30; the return
flight must depart LAX for SFO on 2026-07-13 between 17:00 and 19:30.
Search once each on Google Flights, Kayak, and Momondo, and record
1 most suitable result from each platform with a screenshot.

For lodging, only consider Courtyard by Marriott Santa Monica,
Hampton Inn & Suites Santa Monica, and Hilton Santa Monica Hotel &
Suites. Search Booking.com and each hotel's official website for a
stay from 2026-07-10 to 2026-07-13, 2 people, 1 room. Record room
type, 3-night total price, whether taxes/fees are included,
cancellation policy, rating/address, and screenshots.

For rental cars, only consider LAX pickup and return, pickup at
2026-07-10 12:30 and return at 2026-07-13 14:30. Search Enterprise
for Economy, Compact, and Midsize. On Turo, record only the 2 cheapest
qualifying cars in the search results, without logging in. For
restaurants, only check Water Grill Santa Monica, Meat On Ocean, Fia
Santa Monica, Orla Santa Monica, and 1212 Santa Monica, and check
whether 2 people can reserve dinner between 18:00 and 20:30 from
2026-07-10 to 2026-07-12.

Finally generate `/tmp_workspace/results/santa_monica_trip_plan.md`,
including a daily itinerary, a budget table for flights / hotel /
rental car / restaurants / parking / gas / activity contingency, and
two options: budget-saving and comfortable. Try to keep the
comfortable option's total budget within \$3,200 / 2 people.
\end{clawcode}

\subsection{Multimodal Understanding}\label{app:examples:multimodal}

Tasks here require extracting, interpreting, and generating
information grounded in real images, videos, or audio. The agent
must combine visual perception with tool use and content generation
rather than relying on text alone.

\begin{clawcode}[title={\texttt{task\_01\_scaling\_laws\_figure5\_aspect\_ratio}}]
Download the paper "Scaling Laws for Neural Language Models" from
arXiv, locate the middle "Aspect Ratio" line chart in Figure 5, and
faithfully recreate it with Python + matplotlib.

Requirements:
1. You must find the correct paper yourself and confirm the correct
   page/figure number; do not recreate the wrong chart.
2. The figure should preserve the original axis meanings, logarithmic
   x-axis, three curves for different model sizes, legend, and overall
   style.
3. Perform at least one "draw the chart, compare it with the original,
   then revise" iteration instead of producing it in one pass.
4. Save the final deliverables under `/tmp_workspace/results/`,
   including at least:
   - `figure5_aspect_ratio_recreated.png`
   - `figure5_aspect_ratio_recreated.py`
   - `notes.md` (briefly state which paper and figure you confirmed,
     and what revisions you made)
\end{clawcode}

\begin{clawcode}[title={\texttt{task\_22\_met\_art\_room\_match}}]
Please open the collection pages on The Met website for the following
three paintings:

1. Claude Monet -- https://www.metmuseum.org/art/collection/search/437133
2. Vincent van Gogh -- https://www.metmuseum.org/art/collection/search/436535
3. Caspar David Friedrich -- https://www.metmuseum.org/art/collection/search/438417

Please do the following:

1. Save at least 1 webpage screenshot for each painting to
   `/tmp_workspace/results/artwork_screenshots/`; the screenshot must
   include both the main image and a clear metadata area. If a single
   screenshot cannot fit both, save an additional supplemental
   screenshot for the same artwork and mark that clearly in the
   filename or notes.
2. Read `/tmp_workspace/clawbench/sources/my_room_style.json`.
3. Generate the following in `/tmp_workspace/results/`:
   - `artworks_metadata.csv`
   - `visual_analysis.md`
   - `best_choice_for_my_room.md`
4. `artworks_metadata.csv` must organize at least these fields:
   - artwork_url, title, artist, object_date, medium, dimensions
5. `visual_analysis.md` must analyze each painting's:
   - Main color palette and warm/cool relationship
   - Composition
   - Brushwork or surface texture characteristics
   - Overall atmosphere
6. `best_choice_for_my_room.md` must clearly select the one painting
   best suited to hang in my room, match the artwork's visual
   characteristics to my room conditions point by point, and explain
   why the other two were not selected.
\end{clawcode}

\subsection{Cross-Platform}\label{app:examples:cross-platform}

Tasks here require synchronizing state across heterogeneous
applications and interfaces -- Platform CLI tools like GitHub CLI, web pages, desktop GUI applications,
local files, calendars, citation managers, and so on. Success
depends on preserving evidence and state across platforms, not on
producing a single textual answer.

\begin{clawcode}[title={\texttt{task\_01\_rag\_survey\_gui\_zotero\_obsidian}}]
I have a local PDF from a real RAG survey reading pack and I want it
moved through a real desktop GUI workflow using Zotero and Obsidian.

The PDF is available here:
    /tmp_workspace/clawbench/sources/rag_survey_pack/rag_survey.pdf

Please use the real desktop applications, not a web mock and not just
command-line file editing. A setup service installs/verifies Zotero
and Obsidian before you start; if they are still settling, wait
briefly and try launching them again.

- Open and read the PDF with a visible PDF reader or browser PDF
  viewer.
- Launch the real Zotero desktop app. Create one Zotero record for
  the PDF, including the title, authors, year, venue, DOI or arXiv
  ID, citation key, tags, and a useful abstract/summary. Attach the
  local PDF to that Zotero record.
- Export the Zotero item to BibTeX or Better BibTeX-style `.bib` if
  available. The exported citation key should be `gao2024retrieval`.
- Launch the real Obsidian desktop app. Create/open an Obsidian vault
  under `/tmp_workspace/results/rag_survey_obsidian_vault/` and
  create a literature note that links to the Zotero
  record/citation key. The note must capture the paper's objective,
  method, dataset/corpus or review scope, metrics or evaluation
  dimensions, key findings, limitations, and how we could use it in
  a RAG evaluation plan.

At the end I need these files under `/tmp_workspace/results/`:

- `rag_survey_note_export.md`
- `zotero_rag_survey_export.bib`
- the literature note .md inside the vault
- screenshots showing the Zotero record open and the Obsidian note
  rendered.
\end{clawcode}

\begin{clawcode}[title={\texttt{task\_03\_rust\_tokyo\_meetup\_gui\_calendar}}]
Use real public web pages to organize the Rust Global: Tokyo event
information, then create a reminder event in a real local desktop
calendar GUI.

Verify the information from these real web pages. Do not use a local
simulated site or local mirror page:

- Rust Foundation event page:
  https://rustfoundation.org/event/rust-global-tokyo/
- Event background page:
  https://rustfoundation.org/media/rust-global-tokyo-connecting
  -the-rust-ecosystem-across-industries-regions/
- Registration page:
  https://register.linuxfoundation.org/event/rust-global-tokyo-2025/register
- Venue/travel page:
  https://events.linuxfoundation.org/open-source-summit-japan/attend/venue-travel/

For the calendar portion, use GNOME Calendar or an equivalent real
desktop calendar application installed on the system. Do not use
Calendar Mock, and do not only hand-write a calendar file.

Requirements:
1. Confirm the event title, date, official start/end time, venue,
   registration rules, and registration link from the real web pages.
2. Create an event in the real calendar GUI. The title must include
   `Rust Global: Tokyo`.
3. Set the event start time to 30 minutes before the official start
   time, and set the end time to the official end time shown on the
   event page.
4. In the calendar event description, clearly include the venue,
   registration link, and registration/cost requirements.
5. Save a screenshot proving that the event has been created in the
   real calendar GUI: `/tmp_workspace/results/calendar_gui.png`; if
   the calendar supports export, also save
   `/tmp_workspace/results/rust_global_tokyo.ics`. An ICS import
   preview, a screen where no calendar has been selected, or a dialog
   where import/save has not been clicked does not count as a created
   event. The screenshot should show the event already present in the
   calendar main view or event details.
6. Also write an audit JSON file to
   `/tmp_workspace/results/calendar_evidence.json`. Record the
   calendar application used, event title, start/end time, timezone,
   venue, registration link, and evidence file paths. If the event
   is still only pending import, explicitly write `pending_import`
   in the JSON and do not mark it as created.
7. Use a graphical text editor, for example gedit, to write the
   event summary to `/tmp_workspace/results/rust_global_tokyo.md`.
   Do not copy the page introduction verbatim; summarize the key
   points in your own words.
\end{clawcode}
