# Supplementary material for: UniClawBench: A Universal Benchmark for Proactive Agents on Real-World Tasks
Source: arXiv:2607.08768 source file (2026-07-09)
Supplement: Supplementary file 4 [file D_case_study.tex]

We trace one full attempt of \texttt{task\_09\_loc\_rights\_images},
an exploration task that the executor solved in two cycles after a
corrective user follow-up. The attempt closed at
\texttt{finalScore = 0.96} (\texttt{finalStatus = pass}). Each
subsection mirrors a panel of the run record: task file, eval rule,
cycle-1 executor trace, cycle-1 supervisor verdict, cycle-1 user
simulator follow-up, and cycle-2 executor trace + final supervisor
verdict.

\subsection{Task File}\label{app:case-study:task}

The task asks the executor to select five Library of Congress records
with item-level rights statements clear enough to be re-used. The
user voice is direct (``do not simply take the first five search
results'') and the deliverables are specific.

\begin{clawcode}[title={Task YAML (\texttt{task\_009\_loc\_rights\_images})},label={lst:case:yaml}]
task_id: task_009_loc_rights_images
category: exploration
agent_sys: openclaw
agent_id: main
model: claude-opus-4.6
timeout_seconds: 1200
max_total_seconds: 1800
success_threshold: 0.9

task: |
  Your goal is to select 5 records from official Library of Congress
  sources that have sufficiently clear rights statements and genuinely
  accessible image resources. Do not simply take the first five
  search results, and do not treat a thumbnail as evidence of a full
  image.

  Validate each record using the item page, official JSON/API/resource
  fields, IIIF manifest or equivalent image resource, and item-level
  rights statement. Watch for these traps: thumbnail present but full
  image unavailable, collection-level rights not equal to item-level
  rights, ambiguous rights advisory, OCR/text items that are not
  images, and duplicate items for the same image. Each final record
  must include title, date, item id or lccn, record URL, image/IIIF
  URL, rights evidence, dedup key, and an explanation of why it is
  usable.

  Save:
  - `/tmp_workspace/results/fetch_loc_rights_images.py`
  - `/tmp_workspace/results/loc_rights_images.json`
  - `/tmp_workspace/results/loc_image_exclusions.json`
  - `/tmp_workspace/results/loc_images_notes.json`
  - `/tmp_workspace/results/fetch_loc_rights_images_run.log`.

references:
  - references/eval_rule.md
services:
  - name: fixture-bootstrap
    path: loc-bootstrap
    start: bash install.sh
codex:
  max_user_followups: 2
\end{clawcode}

\subsection{Eval Rule}\label{app:case-study:eval}

The hidden \texttt{eval\_rule.md} for this task follows the schema in
Appendix~\ref{app:format:eval}. We reproduce \S5 (rubric weights) and
\S6 (score caps) below; the supervisor scores using \emph{only} these
lines.

\begin{clawcode}[title={Eval rule \S5 -- checkpoint rubric},label={lst:case:eval5}]
## 5. Checkpoint Rubric

Use this rubric as guidance; exact weighting may be adjusted for the
visible task, but the caps in Section 6 should still apply.

1. Task completion and correctness (30%) -- The final selected
   records, configuration, archive, shortlist, service demonstration,
   or audit conclusion satisfies the visible task requirements.
2. Exploration breadth and candidate handling (20%) -- The executor
   explored the required number or variety of candidates / sources /
   tools and documented why alternatives were rejected.
3. Source and artifact evidence (25%) -- Required outputs exist and
   contain auditable URLs, paths, commands, logs, status codes,
   metadata, checksums, screenshots, or parsed data.
4. Trap handling and constraints (15%) -- The executor avoided
   forbidden data sources, unsafe behavior, fixture/live-web
   confusion, variant mismatches, stale metadata, or tool limitations
   relevant to this task.
5. Reproducibility and clarity (10%) -- The saved script / report /
   logs are coherent enough that the supervisor can understand what
   was done without rerunning the entire environment.

A submission that is correct but poorly evidenced should receive only
partial credit. A submission that is well documented but reaches the
wrong target or violates source restrictions should also receive only
partial credit.
\end{clawcode}

\begin{clawcode}[title={Eval rule \S6 -- score caps},label={lst:case:eval6}]
## 6. Scoring Policy / Caps

Apply these task-specific caps before assigning the final score:

- Cap 0.40 if results are simply the first five search hits.
- Cap 0.55 if thumbnails are treated as full image evidence.
- Cap 0.70 if rights statements are unclear or not tied to official
  LOC pages.

General caps also apply:

- Cap 0.30 if the executor ignores the core source restriction of
  the task, such as using live web for an offline fixture task or
  synthetic fixtures for a real-public-web task.
- Cap 0.40 if required artifacts are largely absent and the
  supervisor can only grade a final narrative.
- Cap 0.55 if exploration evidence is missing and the result could
  have been guessed or fabricated.
- Cap 0.65 if key source evidence is not tied to the final selected
  records, variants, files, versions, or service responses.
- Cap 0.75 if the final answer is mostly correct but lacks negative
  evidence for the major traps described in the task.
- Cap 0.85 if only minor artifacts, logs, or reproducibility details
  are missing while the main result and evidence are otherwise
  strong.

Scores near 1.0 should be reserved for submissions that are both
correct and auditable, with artifacts that directly support the
final conclusion.
\end{clawcode}

\subsection{Cycle 1 -- Executor Trace}\label{app:case-study:trace1}

Table~\ref{tbl:case:trace1} summarizes the first eight assistant
turns of cycle 1. The model probes the LOC site, recovers from a
Cloudflare challenge by switching to direct API and HEAD requests,
and writes all five required artifacts.

\begin{table}[h]
\centering
\small
\begin{tabular}{rlp{0.50\linewidth}}
\toprule
Turn & Tool calls & What the model did \\
\midrule
1 & \texttt{read} & Reads \texttt{SKILL.md} for the agent-browser skill. \\
2 & \texttt{exec} \texttt{mkdir} & ``Now let me research the LOC API to understand how to find items with clear rights and accessible images.'' \\
3 & \texttt{exec} \texttt{agent-browser open} & Opens an LOC search page filtered to image media + public-domain rights. \\
4 & \texttt{exec} \texttt{agent-browser snapshot} & Tries to take a DOM snapshot. \\
5 & \texttt{exec} \texttt{sleep + snapshot} & ``Cloudflare challenge. Let me wait and try again, or use the API directly.'' \\
6 & \texttt{process} & Inspects the running browser process. \\
7 & \texttt{exec} \texttt{curl} & Switches to the LOC JSON API directly via \texttt{curl}, bypassing Cloudflare. \\
8 & \texttt{exec} \texttt{curl -I} & HEAD requests against the LOC tile / IIIF service to verify full image resources actually resolve. \\
\bottomrule
\end{tabular}
\vspace{5pt}
\caption{Cycle 1 first eight executor turns. The model recovers from the Cloudflare block by switching probe strategy without giving up.}\label{tbl:case:trace1}
\end{table}

The remaining turns (not shown) read item-level JSON for each
candidate, normalize titles and dates, dedup by image stem, and write
\texttt{loc\_rights\_images.json}, \texttt{loc\_image\_exclusions.json},
methodology notes, the Python script, and the run log.

\subsection{Cycle 1 -- Supervisor Verdict}\label{app:case-study:verdict1}

The supervisor receives the executor's full visible trajectory plus
the hidden eval rule and ground truth, and emits one structured
decision.

\begin{clawcode}[title={Cycle 1 supervisor verdict (\texttt{score=0.65}, verdict \texttt{continue})},label={lst:case:verdict1}]
verdict: continue
attempt_state: complete_but_failed
recoverable: true
score: 0.65
confidence: high
rationale: |
  All required artifacts are present, and the visible evidence shows
  real LOC exploration via official LOC API endpoints plus direct
  image / IIIF checks. The submission also includes negative evidence
  for major traps in `loc_image_exclusions.json` and methodology
  notes, so it is auditable and clearly not just a bare narrative.

  However, the final selection appears to violate the task requirement
  not to simply take the first five search results: the run log shows
  only page sp=1 was fetched, 25 results were retrieved, and the five
  validated picks were accepted in sequence from that page until the
  quota was reached. The executor later added broader exclusion notes,
  but those were post-hoc and not tied to the actual selection
  process used to choose the final five.

  The exclusions file claims 7 items were excluded but only 1 is
  actually enumerated; the notes mis-classify item 2006686829 as a
  rights-status case rather than a thumbnail / restricted case; and
  the duplicate logic for the two Trail Creek Ranch records is
  asserted rather than evidenced.

  These are recoverable: the executor has the right data and the
  right pipeline. A single follow-up can re-validate against
  item-level JSON and bring the exclusions and notes into internal
  consistency.

missing_artifacts: []
guidance_tags: ["fix_internal_consistency", "broaden_candidate_pool"]
\end{clawcode}

\subsection{Cycle 1 -- User Simulator Follow-up}\label{app:case-study:userturn}

Because the verdict is \texttt{continue}, the runner launches the
user simulator. From the supervisor it receives only a four-field
handoff -- verdict, attempt state, recoverability, and score
(Appendix~\ref{lst:case:handoff}); the supervisor's
\texttt{rationale}, \texttt{missing\_artifacts}, and
\texttt{guidance\_tags} are never forwarded, and the hidden eval
rule is not mounted into the user simulator's workspace. Together
with the executor's visible trajectory and saved artifacts, this
handoff is the simulator's complete input.

\begin{clawcode}[title={\texttt{user\_handoff} (cycle 1)},label={lst:case:handoff}]
user_handoff = {
    "verdict":        "continue",
    "attempt_state":  "complete_but_failed",
    "recoverable":    true,
    "score":          0.65
}
\end{clawcode}

The user simulator's output, after a deterministic post-rewrite step,
is the message in Appendix~\ref{lst:case:userturn}, sent to the
executor as the next user turn.

\begin{clawcode}[title={Cycle 1 user simulator follow-up (verbatim)},label={lst:case:userturn}]
Please fix the results by re-validating with official item JSON /
item pages and replacing anything that was inferred from just the
first API page.

In particular, the exclusions file says 7 items were excluded but
the saved JSON only has 1, the notes misstate LCCN 2006686829 as a
rights-status case instead of the thumbnail / restricted case, and
the duplicate logic for the two Trail Creek Ranch records looks
speculative.

Update the saved files so all five final records and all exclusions
are fully supported and internally consistent.
\end{clawcode}

\subsection{Cycle 2 -- Executor Trace}\label{app:case-study:trace2}

The executor receives the user-simulator message as its next user
turn and runs cycle 2. Table~\ref{tbl:case:trace2} summarizes the
ten assistant turns; the model now drives a tightened pipeline that
re-fetches official item JSON for each candidate, discovers two
substantive errors that even the user message had not named, and
regenerates all five output files from the corrected pipeline.

\subsection{Cycle 2 -- Supervisor Verdict}\label{app:case-study:verdict2}

The supervisor's second decision pushes the score from 0.65 to 0.96,
crossing the rubric's pass band.

The runner records \texttt{finalScore = 0.96}. The user simulator is
not invoked again on a \texttt{pass} verdict, and the attempt closes
after exactly two cycles.

\begin{table}[t]
\centering
\small
\begin{tabular}{rlp{0.50\linewidth}}
\toprule
Turn & Tool calls & What the model did \\
\midrule
1 & \texttt{exec} \texttt{cat} & Reads back its own existing \texttt{loc\_image\_exclusions.json} to confirm the inconsistency the user described. \\
2 & \texttt{exec} \texttt{python3} & ``The issues are: (1) exclusions file has 7 hand-written entries the script never produced; (2) LCCN 2006686829 is described incorrectly; ...'' Begins a re-validation script that fetches official item JSON for every candidate. \\
3 & \texttt{exec} \texttt{python3} & ``I see an important issue with the Koussevitzky item: its \texttt{rights\_advisory} field is \texttt{N/A}\dots'' Discovers a real issue the user message had not flagged. \\
4 & \texttt{process} & Inspects the running fetch process. \\
5 & \texttt{exec} \texttt{python3} & ``Now I have complete, verified data from the official item JSONs. Key findings: Koussevitzky's \texttt{rights\_advisory} is \texttt{FIELD\_MISSING} \dots'' \\
6 & \texttt{write} & ``The Feraille-o item IS a digitized card catalog, not an audio recording.'' Writes the corrected \texttt{fetch\_loc\_rights\_images.py}. \\
7 & \makecell[l]{\texttt{exec python3} \\ \texttt{fetch\_loc\_rights\_images.py}} & Runs the corrected pipeline; produces a fresh selection of 5, exclusions = 7, with item-JSON-grounded evidence for every record. \\
8 & \makecell[l]{\texttt{exec} \\ \texttt{cat loc\_rights\_images.json}} & Verifies the new selection. \\
9 & \makecell[l]{\texttt{exec} \\ \texttt{cat loc\_image\_exclusions.json}} & Verifies the new exclusions. \\
10 & \makecell[l]{\texttt{exec} \\ \texttt{cat loc\_images\_notes.json}} & Verifies the regenerated methodology notes. \\
\bottomrule
\end{tabular}
\vspace{5pt}
\caption{Cycle 2 executor turns. The model goes beyond the user's stated complaints, finding two additional grounded issues (Koussevitzky rights field, Feraille-o item type) and rebuilding the pipeline rather than patching the saved files in place.}\label{tbl:case:trace2}
\end{table}

\begin{clawcode}[title={Cycle 2 supervisor verdict (\texttt{score=0.96}, verdict \texttt{pass})},label={lst:case:verdict2}]
verdict: pass
attempt_state: complete_and_passed
recoverable: false
score: 0.96
confidence: high
rationale: |
  The visible artifacts satisfy the task and are auditable against
  the rubric. All required outputs are present in `visible/result/`.
  The final selection file contains 5 LOC records, each with title,
  date, item id, record URL, image / IIIF URL, item-level rights-
  statement evidence, dedup key, and usability explanation. The run
  log ties each selected record to an official LOC item JSON URL,
  records access_restricted: false, records the item-level
  rights_advisory, and shows image verification via HTTP HEAD with
  content type and byte size. The Highsmith item also includes IIIF
  evidence. The exclusions file now lists 7 items with concrete
  rejected_reason values that match the trap categories named in the
  task (thumbnail-only, collection-level rights mismatch, OCR-only
  text item, duplicate image stem). Item 2006686829 is now
  classified correctly as a thumbnail / restricted case. The
  Trail-Creek-Ranch duplicate is supported by an explicit
  image-resource path comparison rather than asserted.

  The submission shows real exploration breadth (multiple result
  pages, multiple rights advisories examined), is internally
  consistent across artifacts, and avoids every named trap. A small
  amount of supporting commentary in `loc_images_notes.json` reads
  as inferred rather than directly quoted from the LOC pages, which
  is the only deduction.

missing_artifacts: []
guidance_tags: []
\end{clawcode}

\subsection{What This Trace Demonstrates}\label{app:case-study:lessons}

Three properties of the closed-loop design from the main paper are
visible in this single attempt:

\begin{enumerate}
  \item \textbf{The supervisor catches recoverable failure modes
  rather than rejecting them outright.} Cycle 1 has the right
  pipeline and the right data; only the selection rigor and the
  exclusion-file consistency are insufficient. Returning
  \texttt{continue} (not \texttt{fail}) at \texttt{score = 0.65}
  preserves the executor's progress while flagging the remediable
  gap.
  \item \textbf{The information firewall is structural, not
  stylistic.} The supervisor returns a seven-field decision but
  only four fields cross to the user simulator
  (Appendix~\ref{app:case-study:userturn}). Hidden judging assets are
  never mounted into the user simulator's workspace, and a
  deterministic rewriter further sanitizes the simulator's
  candidate text. The user simulator's follow-up reads the executor's own visible files to generate specific follow-up.
  \item \textbf{Multi-turn recovery is a core capability.} The
  cycle-1 score of 0.65 would have been a fail under any single-turn
  paradigm; cycle 2 reaches 0.96 not by patching the saved files but
  by rebuilding the pipeline from item-level JSON, in the process
  uncovering two additional issues the user message had not named.
  UniClawBench scores reflect both the model's first-pass and its
  recovery capabilities.
\end{enumerate}
